# Supplementary material for: Situated Conditional Reasoning
Source: arXiv:2109.01552 source file (2023-04-17)
Supplement: Supplementary file 2 [file macros.tex]

%%%%%%%%%%%%%%%%%%%%%%%%%%%%%%%%%%%%%%%%%%%%%%%%%%
% Begin macro definitions
%%%%%%%%%%%%%%%%%%%%%%%%%%%%%%%%%%%%%%%%%%%%%%%%%%
\usepackage{amssymb}
\usepackage{amsmath}
\usepackage{stmaryrd}
\usepackage{mathrsfs} 
\usepackage{comment}
\usepackage{xcolor}

\usepackage{soul}
\usepackage{url}
\usepackage[hidelinks]{hyperref}
%\usepackage{graphicx}
\usepackage{amsmath}
\usepackage{amsthm}
\usepackage{booktabs}
%\usepackage{algorithm}
%\usepackage{algorithmic}
\urlstyle{same}
\usepackage{comment}
\usepackage{latexsym} 

\frenchspacing  %Required

\newcommand{\remaindent}{\ensuremath{\hspace{-0.1cm}\Downarrow\hspace{-0.1cm}}}
\newcommand{\lent}{\ensuremath{\leq_e}}
\newcommand{\gent}{\ensuremath{\geq_e}}
\newcommand{\equivent}{\ensuremath{\equiv_e}}
\newcommand{\lessent}{\ensuremath{<_e}}
\renewcommand{\L}{\ensuremath{\mathfrak{L}}}


\usepackage{amsfonts}
\usepackage[utf8]{inputenc}
\usepackage[thinlines]{easytable}
%\usepackage[ruled,linesnumbered,vlined,scleft]{algorithm2e}
%\usepackage[commentsnumbered,linesnumbered]{algorithm2e}
\usepackage{subfigure}
\usepackage{color}








%%%%%%%%%%%%%%%%%%%%%%%%%%%%%%%%%%%%%%%%%%%%%%%%%%
% General expressions and commands:

\newcommand{\ie}{\mbox{i.e.}}
\newcommand{\eg}{\mbox{e.g.}}
\newcommand{\cf}{\mbox{cf.}}
\newcommand{\viz}{\mbox{viz.}}
\newcommand{\wrt}{\mbox{w.r.t.}}
\newcommand{\stt}{\mbox{s.t.}}
\newcommand{\wolog}{\mbox{w.l.o.g.}}
\newcommand{\etal}{\mbox{et al}}
\newcommand{\vs}{\mbox{vs.}}
\newcommand{\aka}{\mbox{a.k.a.}}
\newcommand{\myskip}{\medskip} % space interlines
\newcommand{\ol}[1]{\overline{#1}}
\newcommand{\df}[1]{\textbf{#1}} % to emphasise defined terms in definitions

%%%%%%%%%%%%%%%%%%%%%%%%%%%%%%%%%%%%%%%%%%%%%%%%%%
% Mathematical general expressions:

%\newcommand{\qed}{\rule{2mm}{2mm}}
\newcommand{\tuple}[1]{\langle #1 \rangle}
\newcommand{\defined}{\:\raisebox{1ex}{\scalebox{0.5}{\ensuremath{\mathrm{def}}}}\hskip-1.65ex\raisebox{-0.1ex}{\ensuremath{=}}\:}
\newcommand{\abbrev}{\mathrel{\mathop:}=}
\newcommand{\eqclass}[1]{[#1]} % equivalence class of an element
\newcommand{\assigned}{\mathrel{\mathop:}=}
\newcommand{\grammar}{\mathrel{\mathop:}\assigned}

%%%%%%%%%%%%%%%%%%%%%%%%%%%%%%%%%%%%%%%%%%%%%%%%%%
% Theorem-like environments:

%\newtheorem{definition}{Definition}
%\let\olddefinition\definition
%\renewcommand{\definition}{\olddefinition\normalfont}

%\newtheorem{lemma}{Lemma}%[section]
%\newtheorem{theorem}{Theorem}%[section] 
%\newtheorem{proposition}{Proposition}%[section]
%\newtheorem{corollary}{Corollary}%[section]

%\newtheorem{example}{Example}%[section]%}
%\let\oldexample\example
%\renewcommand{\example}{\oldexample\normalfont}

%\newtheorem{remark}{Remark}%[section]
\newtheorem{observation}{Observation}%[section]
%\newenvironment{proof}{\noindent\textbf{Proof:}\null\hfill\null\newline}{\hfill\qed}

%%%%%%%%%%%%%%%%%%%%%%%%%%%%%%%%%%%%%%%%%%%%%%%%%%
% Computational complexity:

\newcommand{\ptime}{\textsc{P}}
\newcommand{\np}{\textsc{NP}}
\newcommand{\exptime}{\textsc{exptime}}
\newcommand{\pspace}{\textsc{pspace}}
\newcommand{\npcomplete}{\textsc{np-complete}}

%%%%%%%%%%%%%%%%%%%%%%%%%%%%%%%%%%%%%%%%%%%%%%%%%%
% Sets and set operations:

% Set union: \cup, Set intersection: \cap, Set difference: \setminus
\newcommand{\powerset}[1]{\mathscr{P}(#1)} % powerset
\newcommand{\symdiff}{\dotdiv} % symmetric difference

%%%%%%%%%%%%%%%%%%%%%%%%%%%%%%%%%%%%%%%%%%%%%%%%%%
% Special sets:

% Language:
\newcommand{\Prp}{\ensuremath{\mathcal{P}}}
\newcommand{\Lang}{\ensuremath{\mathcal{L}}}

% Theories, signature:
\newcommand{\T}{\ensuremath{\mathcal{T}}} % a theory
\newcommand{\KB}{\ensuremath{\mathcal{K}}} % a knowledge base
\newcommand{\B}{\ensuremath{\mathcal{B}}} % defeasible belief set
\newcommand{\DS}{\ensuremath{\mathcal{D}}} % a defeasible set
\newcommand{\Sig}{\ensuremath{\mathcal{S}}} % a set of atoms, or a signature
% Theories, signature:
\newcommand{\A}{\ensuremath{\mathcal{A}}} % an ABox
\newcommand{\calO}{\ensuremath{\mathcal{K}_\mathcal{I}}}% a set of individuals
%%%%%%%%%%%%%%%%%%%%%%%%%%%%%%%%%%%%%%%%%%%%%%%%%%
% Logical connectives and meta-logical basic definitions:

% Logical negation: \lnot, Logical conjunction: \land, Logical disjunction: \lor
\newcommand{\limp}{\rightarrow} % logical implication
\newcommand{\liff}{\leftrightarrow} % biconditional
\newcommand{\lexor}{\oplus} % exclusive or

% Entailment  in a class of models:
\newcommand{\Centails}[1]{\models_{\raisebox{-0.25ex}{$\!\!\!_{#1}$}}\!\!}
\newcommand{\nCentails}{\not\Centails}

% Provable in a given logical system:
\newcommand{\provable}[1]{\vdash_{\raisebox{-0.2ex}{$\!\!\!_{#1}$}}\!\!}
\newcommand{\nprovable}[1]{\not\provable{#1}}

%%%%%%%%%%%%%%%%%%%%%%%%%%%%%%%%%%%%%%%%%%%%%%%%%%
% Classical Propositional Logic:

\newcommand{\verum}{\ensuremath{\text{\it true}}}
\newcommand{\falsum}{\ensuremath{\text{\it false}}}
\newcommand{\fml}{\ensuremath{\varphi}} % a classical formula
\newcommand{\clause}{\ensuremath{\chi}} % a clause
\newcommand{\term}{\ensuremath{\pi}} % a term
\newcommand{\Val}{\ensuremath{\mathcal{V}}} % set of propositional valuations
\newcommand{\fm}[1]{\ensuremath{{\sf fml}({#1})}}


% Satisfaction relation:
\newcommand{\sat}{\Vdash}
\newcommand{\nsat}{\not\sat}

% Classical propositional entailment:
\newcommand{\entails}{\models}
\newcommand{\nentails}{\not\entails}
\newcommand{\entailed}{\raisebox{1.1ex}{\rotatebox{180}{$\entails$}}}

% Classical provability:
\newcommand{\proves}{\vdash}
\newcommand{\nproves}{\not\proves}

% Propositional consequence relation and provability:
\newcommand{\CPL}{{\sf CPL}}
\newcommand{\CPLentails}{\Centails{\CPL}}
\newcommand{\nCPLentails}{\not\CPLentails}
\newcommand{\CPLtheorem}{\provable{\CPL}}
\newcommand{\nCPLtheorem}{\not\CPLtheorem}

%%%%%%%%%%%%%%%%%%%%%%%%%%%%%%%%%%%%%%%%%%%%%%%%%%
% Modal logic:

% Modal operators:
\newcommand{\nec}{\Box}
\newcommand{\poss}{\Diamond}
\newcommand{\Nec}[1]{[ #1 ]}
\newcommand{\Poss}[1]{\langle #1 \rangle}
\newcommand{\obl}{\scalebox{0.75}{\raisebox{0.5ex}{\ensuremath{\bigcirc}}}} % obligation

% Kripke models:
\newcommand{\W}{\ensuremath{\text{\it W}}} % possible worlds
\newcommand{\R}{\ensuremath{\text{\it R}}} % accessibility relation
\newcommand{\V}{\ensuremath{\text{\it V}}} % valuation function
\newcommand{\M}{\mathscr{M}}
\newcommand{\MSet}{\ensuremath{\mathcal{M}}} % set of models
\newcommand{\U}{\mathcal{U}} % set of pointed models

% Valid in a given model:
\newcommand{\Mvalid}[1]{\models^{\raisebox{-0.3ex}{$\!\!\!^{#1}$}}\!\!}
\newcommand{\nMvalid}[1]{\not\Mvalid{#1}}

% Modal logic K:
\newcommand{\K}{{\sf K}}
\newcommand{\Kentails}{\Centails{\K}}
\newcommand{\nKentails}{\not\Kentails}
\newcommand{\Ktheorem}{\provable{\K}}
\newcommand{\nKtheorem}{\not\Ktheorem}
\newcommand{\schemaK}{\ensuremath{\text{{\it K}}}}
\newcommand{\ruleRN}{\ensuremath{\text{{\it RN}}}}

%%%%%%%%%%%%%%%%%%%%%%%%%%%%%%%%%%%%%%%%%%%%%%%%%%
% Description Logics:

\newcommand{\N}{\ensuremath{{\sf N}}} % set of concept names
\newcommand{\CN}{\ensuremath{{\sf N}_{\mathscr{C}}}} % set of concept names
\newcommand{\RN}{\ensuremath{{\sf N}_{\mathscr{R}}}} % set of role names
\newcommand{\IN}{\ensuremath{{\sf N}_{\mathscr{I}}}} % set of individual names
\newcommand{\Names}{\ensuremath{{\sf N}}}  % union of both (the whole signature)
\newcommand{\dlAnd}{\sqcap}
\newcommand{\dlOr}{\sqcup}
\newcommand{\subs}{\sqsubseteq}
\newcommand{\nsubs}{\not\subs}
\newcommand{\I}{\ensuremath{\mathcal{I}}}
\newcommand{\J}{\ensuremath{\mathcal{J}}}
\newcommand{\Iof}[1]{{#1}^{\I}}
\newcommand{\Db}{\mathcal{D}}
\newcommand{\Dom}{\Delta}
\newcommand{\Ifunc}{\Iof{\cdot}}
\newcommand{\ALC}{\ensuremath{\mathcal{ALC}}}
\newcommand{\SHIF}{\ensuremath{\mathcal{SHIF}}}
\newcommand{\SHOIN}{\ensuremath{\mathcal{SHOIN}}}
\newcommand{\EL}{\ensuremath{\mathcal{EL}}}
\newcommand{\inv}{^{-}} % for role inverse roles
\newcommand{\ABox}{\ensuremath{\mathcal{A}}}
\newcommand{\Ont}{\ensuremath{\mathcal{O}}}

\newcommand{\C}{\ensuremath{\mathcal{C}}}


% Concept and role names:
\newcommand{\NPP}{{\sf NuclearPP}}
\newcommand{\AtomicPile}{{\sf AtomicPile}}
\newcommand{\rNPP}{{\sf RiskyNPP}}
\newcommand{\BrNPP}{{\sf BrazilianNPP}}
\newcommand{\Brazil}{{\sf Brazil}}
\newcommand{\Safe}{{\sf Safe}}
\newcommand{\SeismicArea}{{\sf SeismicArea}}
\newcommand{\isLocated}{{\sf isLocated}}
\newcommand{\hasComponent}{{\sf hasComponent}}
\newcommand{\meltDown}{{\sf meltDown}}
\newcommand{\marriedTo}{{\sf marriedTo}}
\newcommand{\partOf}{{\sf partOf}}
\newcommand{\parentOf}{{\sf parentOf}}
\newcommand{\progenitorOf}{{\sf progenitorOf}}
\newcommand{\worksFor}{{\sf worksFor}}
%\newcommand{\bird}{{\sf b}}
%\newcommand{\penguin}{{\sf p}}
%\newcommand{\flies}{{\sf f}}
\newcommand{\wings}{{\sf w}}
\newcommand{\nbird}{\overline{\sf b}}
\newcommand{\npenguin}{\overline{\sf p}}
\newcommand{\nflies}{\overline{\sf f}}
\newcommand{\nwings}{\overline{\sf w}}
\newcommand{\p}{\sf p}
\newcommand{\q}{\sf q}
\newcommand{\rr}{\sf r}
\newcommand{\notp}{\overline{\sf p}}
\newcommand{\notq}{\overline{\sf q}}
\newcommand{\notr}{\overline{\sf r}}

%%%%%%%%%%%%%%%%%%%%%%%%%%%%%%%%%%%%%%%%%%%%%%%%%%
% Special functions and relations:

% Range of a function or relation:
\newcommand{\range}[1]{{\ensuremath{\text{\it range}(#1)}}}
% Domain of a function or relation:
\newcommand{\domain}[1]{{\ensuremath{\text{\it domain}(#1)}}}
% Atoms of a formula:
\newcommand{\atm}[1]{{\ensuremath{\text{\it atm}(#1)}}}
% Literals of a formula:
\newcommand{\lit}[1]{{\ensuremath{\text{\it lit}(#1)}}}
% Symbols in a formula:
\newcommand{\sig}[1]{{\ensuremath{\text{\it sig}(#1)}}}
% Cardinality of a set:
\newcommand{\card}[1]{{\ensuremath{\text{\it card}(#1)}}}
% Models of a formula:
\newcommand{\Mod}[1]{\llbracket#1\rrbracket}
% Logical consequences of a theory:
\newcommand{\Cn}[1]{{\ensuremath{\text{\it Cn}(#1)}}}
\newcommand{\Cns}[2]{{\ensuremath{\text{\it Cn}_{#1}(#2)}}}

%%%%%%%%%%%%%%%%%%%%%%%%%%%%%%%%%%%%%%%%%%%%%%%%%%
% Defeasible Stuff:

\newcommand{\dentails}{\mid\hskip-0.40ex\approx}
\newcommand{\ndentails}{\not\mid\hskip-0.40ex\approx}
\renewcommand{\bar}[1]{\overline{#1}}
\newcommand{\twiddle}{\mathrel|\joinrel\sim}
\newcommand{\ntwiddle}{\not\twiddle}
%\newcommand{\usually}{\raisebox{-0.5ex}{$\:\stackrel{\sqsubset}{{\scriptstyle\sim}}\:$} }
\newcommand{\usually}{\:\raisebox{0.45ex}{\ensuremath{\sqsubset}}\hskip-1.7ex\raisebox{-0.6ex}{\scalebox{0.9}{\ensuremath{\sim}}}\:}
\newcommand{\nusually}{\not\hspace{-1.1mm}\usually}
%\newcommand{\usuallyeq}{\raisebox{1.5ex}{\rotatebox{180}{$\cong$}}}
%\newcommand{\nusuallyeq}{\not\hspace{-1.1mm}\usuallyeq}
% Preferential models:
\newcommand{\St}{\ensuremath{\text{\it S}}} % set of states
\newcommand{\lab}{\ensuremath{\ell}} % labeling function
\newcommand{\pref}{\prec} % preference relation
\newcommand{\npref}{\not\pref}
\newcommand{\PM}{\mathscr{P}} % preferential model
\newcommand{\RM}{\mathscr{R}} % ranked model
\newcommand{\CM}{\mathscr{C}} % coherent ranked model
\newcommand{\RSet}{\ensuremath{\mathcal{R}}} % set of ranked models
\newcommand{\Rentails}{\Centails{\RSet}} % entailment in the class of ranked models
\newcommand{\nRentails}{\not\Rentails}
\newcommand{\Sat}{\mathrel|\joinrel\equiv} % satisfaction by a state
\newcommand{\nSat}{\not\Sat}
\newcommand{\states}[1]{\llbracket#1\rrbracket} % requires package stmaryrd
\newcommand{\rk}{\ensuremath{\text{\it rk}}} % ranking function
\newcommand{\ri}{\ensuremath{\text{\it r}}} % ranking function
\newcommand{\ei}{\ensuremath{\text{\it e}}} 
\newcommand{\EI}{\ensuremath{\text{\it E}}} 
\newcommand{\ES}{\ensuremath{\mathcal{E}}} 
\newcommand{\nme}{\ensuremath{\mathcal{R}}} % relation of being not more exceptional than
%\newcommand{\C}{\ensuremath{\mathscr{C}}} % set of consistent concepts
\newcommand{\RC}{\ensuremath{\mathcal{R}^{\twiddle}}} % rational closure
\newcommand{\rel}{\ensuremath{\text{\it R}}} % binary relation on the domain
\newcommand{\sel}{{\ensuremath{\text{\sf sel}}}} % selection function

\newcommand{\OI}{\ensuremath{\mathcal{O}}} % ordered interpretation
\newcommand{\PI}{\ensuremath{\mathcal{P}}} % preferential interpretation
\newcommand{\RI}{\mathscr{R}} % ranked model
%\newcommand{\RI}{\ensuremath{\mathcal{R}}} % ranked interpretation
\newcommand{\dsrel}{\leadsto}
\newcommand{\ndsrel}{\not\dsrel}
\newcommand{\D}{\ensuremath{\mathcal{D}}} % a defeasible TBox
\newcommand{\Rs}{\mathscr{R}} % set of ranked models with same classical \I
\newcommand{\X}{\mathcal{X}} % variable for defeasible entailment subscript
\newcommand{\generalent}{\entails_{\X}} %subscripted entailment, based on variable \X
\newcommand{\rmax}{\text{rmax}}
\newcommand{\rmin}{\text{rmin}}


% Definitions for flag and flame (defeasible modal operators):
\newcommand*{\myleftmid}{%
      \mathrel{\vcenter{\offinterlineskip
      \vskip-0.25ex\hbox{$\shortmid$}}}}
\newcommand*{\myrightmid}{%
      \mathrel{\vcenter{\offinterlineskip
      \vskip-0.7ex\hbox{$\shortmid$}}}}
\newcommand*{\twosim}{%
      \mathrel{\vcenter{\offinterlineskip
      \vskip0.05ex\hbox{$\sim$}\vskip0.25ex\hbox{$\sim$}}}}
\newcommand{\bartwosim}{\mathrel{\myleftmid}\hskip-0.03ex\joinrel\twosim}
% Defeasible necessity:
\newcommand{\dnec}{\mathrel{\bartwosim}\hskip-.05ex\joinrel\myrightmid}
% Defeasible possibility:
\newcommand{\dposs}{\scalebox{0.8}{\raisebox{-0.2ex}{\rotatebox{57}{\ensuremath{\dnec}}}}\hskip-0.3ex}
% Defeasible obligation:
\newcommand{\smallsim}{\scalebox{0.86}{\raisebox{0.4ex}{\ensuremath{\sim}}}}
\newcommand{\dobl}{\mathrel{\obl}\hskip-1.9ex\joinrel\smallsim\hskip0.2ex}
% Language with defeasible modalities:
\newcommand{\Langd}{\widetilde{\Lang}}
% Defeasible quantifiers:
\newcommand{\smallsimforall}{\scalebox{0.68}{\raisebox{0.76ex}{\ensuremath{\sim}}}}
\newcommand{\dforall}{\forall\hskip-1.06ex\raisebox{0.7ex}{\scalebox{0.7}{\ensuremath{\textcolor{white}{\bullet}}}}\hskip-1.88ex\joinrel\smallsimforall}
\newcommand{\smallsimexists}{\scalebox{0.65}{\raisebox{0.62ex}{\ensuremath{\sim}}}}
\newcommand{\dexists}{\exists\hskip-1.5ex\scalebox{1.2}{\ensuremath{\textcolor{white}{\bullet}}}\hskip-2.05ex\joinrel\smallsimexists}

\newcommand{\ratent}{\vdash_{r}}

\newcommand{\minent}{\entails_R^{\cup}}
\newcommand{\ratentabox}{\vdash_{r}}
\newcommand{\tw}[1]{\widetilde{#1}}
\newcommand{\E}{\ensuremath{\mathcal{E}}} % exceptionality function
\newcommand{\e}{\ensuremath{\varepsilon}} % exceptionality function
%\newtheorem{procedure}{
%[section]

%%%%%%%%%%%%%%%%%%%%%%%%%%%%%%%%%%%%%%%%%%%%%%%%%%
% Miscellaneous:

% Global options:
%\renewcommand{\labelitemi}{{\small\textbullet}}
%\renewcommand\arraystretch{1.5}
%\renewcommand{\familydefault}{\sfdefault} % sets font to sans serif globally 

% Useful commands:
\newcommand{\nil}{\textcolor{white}{a}} 
\newcommand{\hide}[1]{}
\newcommand{\red}[1]{\textcolor{red}{#1}}
%\newcommand{\todo}[1]{\textcolor{red}{\underline{{\sf #1}} $\blacktriangleright$}}
%\newcommand{\note}[1]{\textcolor{green}{\underline{{\sf #1}} $\blacktriangleright$}}
\newcommand{\who}[1]{\textcolor{orange}{\underline{{\sf #1}} $\blacktriangleright$}}
% Rounded white box with orange frame:
\newlength{\RoundedBoxWidth}
\newsavebox{\WhiteRoundedBox}
\newenvironment{WhiteBox}[1][\dimexpr\textwidth-4.5ex]%
   {\setlength{\RoundedBoxWidth}{\dimexpr#1}
    \begin{lrbox}{\WhiteRoundedBox}
       \begin{minipage}{\RoundedBoxWidth}}%
   {   \end{minipage}
    \end{lrbox}
    \begin{center}
    \begin{tikzpicture}%
       \draw node[draw=Orange,fill=white,rounded corners,line width=1.5pt,%
             inner sep=0.7ex,text width=\RoundedBoxWidth]%
             {\usebox{\WhiteRoundedBox}};
    \end{tikzpicture}
    \end{center}}

\newcommand{\cass}[2]{\mbox{$#1:#2$}}
\newcommand{\rass}[3]{\mbox{$(#1,#2):#3$}}



%%%%%%%%%%%%%%%%%%%%%%%%%%%%%%%%%%%%%%%%%%%%%%%%%%%%%%%%%%%%%%%%%%%%%%%%%%%
% Macros for concrete examples:

\newcommand{\avi}{\ensuremath{\mathsf{a}}}
\newcommand{\mam}{\ensuremath{\mathsf{m}}}
\newcommand{\nuc}{\ensuremath{\mathsf{n}}}
\newcommand{\vtb}{\ensuremath{\mathsf{v}}}
\newcommand{\extra}{\ensuremath{\mathsf{e}}}

\newcommand{\ce}[1]{\ensuremath{\mathsf{#1}}}
\renewcommand{\P}{\ensuremath{\mathcal{P}}}

\newcommand{\bird}{\ensuremath{\mathsf{b}}}
\newcommand{\flies}{\ensuremath{\mathsf{f}}}
\newcommand{\peng}{\ensuremath{\mathsf{p}}}
\newcommand{\dodo}{\ensuremath{\mathsf{d}}}
\newcommand{\mc}{\ensuremath{\mathsf{mc}}}

%%%%%%%%%%%%%%%%%%%%%%%%%%%%%%%%%%%%%%%%%%%%%%%%%%%%%%%%%%%%%%%%%%%%%%%%%%%


%%%%%%%%%%%%%%%%%%%%%%%%%%%%%%%%%%%%%%%%%%%%%%%%%%%%%%%%%%%%%%%%%%%%%%%%%%%
% A macro to be used in revised papers
\newcommand{\modify}[1]{\textcolor{black}{#1}}

%%%%%%%%%%%%%%%%%%%%%%%%%%%%%%%%%%%%%%%%%%%%%%%%%%%%%%%%%%%%%%%%%%%%%%%%%%%%
% Environments for AAAI
\newtheorem{example}{Example}
\newtheorem{definition}{Definition}
\newtheorem{theorem}{Theorem}
\newtheorem{corollary}{Corollary}
\newtheorem{proposition}{Proposition}
\newtheorem{lemma}{Lemma}
%%%%%%%%%%%%%%%%%%%%%%%%%%%%%%%%%%%%%%%%%%%%%%%%%%
% End macro definitions
%%%%%%%%%%%%%%%%%%%%%%%%%%%%%%%%%%%%%%%%%%%%%%%%%%
